# Supplementary material for: A Reversible Structural Phase Transition by Electrochemical Ion Injection into a Conjugated Polymer
Source: arXiv:1910.06440 ancillary file (2019-10-14)
Supplement: Supplementary file 1 [file Supplementary_Information.pdf]

Supplementary Information for

# A Reversible Structural Phase Transition by Electrochemical Ion Injection into a Conjugated Polymer

Connor G. Bischak,<sup>1</sup> Lucas Q. Flagg,<sup>1</sup> Kangrong Yan<sup>2</sup>, Tahir Rehman<sup>2</sup>, Daniel W. Davies<sup>3</sup>, Ramsess J. Quezada,<sup>1</sup> Jonathan W. Onorato,<sup>4</sup> Christine K. Luscombe,<sup>4,5</sup> Ying Diao,<sup>3</sup> Chang-Zhi Li,<sup>2</sup> David S. Ginger<sup>1\*</sup>

<sup>1</sup>Department of Chemistry, University of Washington, Seattle, Washington 98195-1700, United States

<sup>2</sup>MOE Key Laboratory of Macromolecular Synthesis and Functionalization, State Key Laboratory of Silicon Materials, Department of Polymer Science and Engineering, Zhejiang University, Hangzhou 310027, P.R. China

<sup>3</sup>Department of Chemical and Biomolecular Engineering, University of Illinois at Urbana-Champaign, 600 South Mathews Avenue, Urbana, Illinois 61801, United States

<sup>4</sup>Department of Materials Science and Engineering, University of Washington, Seattle, Washington 98195, United States

<sup>5</sup>Department of Molecular Engineering and Sciences, University of Washington, Seattle, Washington 98195, United States

## Table of Contents:

1. Materials and Methods
2. Supplementary Text on Diffusion Calculations
3. Supplementary Figures 1-18
4. Supplementary Movie Captions S1-S3
5. Supplementary References

## Materials and Methods

### Synthesis and Characterization of PB2T-TEG

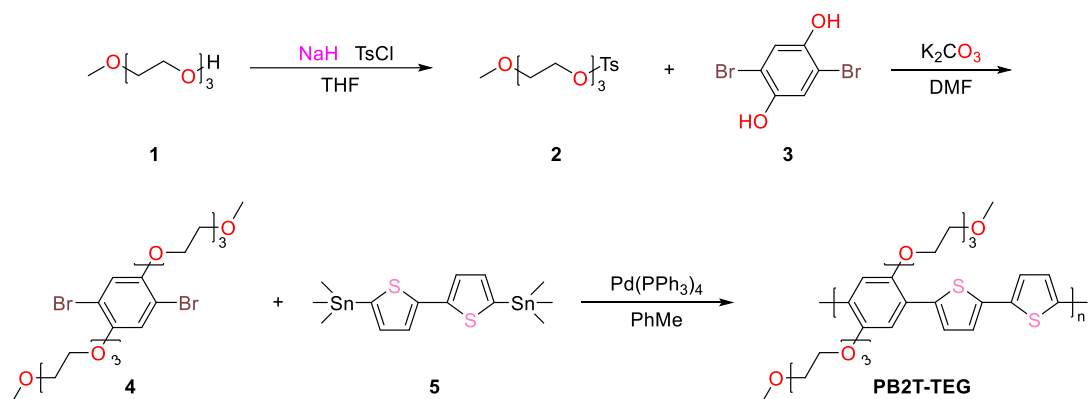

**Scheme 1.** Synthetic procedure for monomer 4 and polymer PB2T-TEG.

<sup>1</sup>H NMR spectra were characterized by Bruker Advance III 400 (FT, DCH Cryoprobe, 400 MHz) and Bruker Advance III 500 (FT, DCH Cryoprobe, 500 MHz) nuclear magnetic resonance (NMR) spectroscopy.

**Compound 2:** The solution of compound 1 (10 g, 0.060 mol) was prepared in dry THF (15 ml) under nitrogen atmosphere. Then 60% suspension of NaH (2.92 g, 0.073 mol) was added into solution at 0 °C. Upon cessation of H<sub>2</sub> evolution, TsCl (11.6 g, 0.061 mol) in THF (10 ml) was added into reaction mixture. The temperature of the reaction mixture was gradually raised to room temperature and stirred overnight. The resulting solution was filtered, the solvent was removed, and crude oil further purified by silica gel chromatography (EtOAc/PE) (14 g, 72%). <sup>1</sup>H NMR (500 MHz, CDCl<sub>3</sub>) δ 7.81-7.79 (m, 2H), 7.34 (d, 2H), 4.17-4.15 (m, 2H), 3.70-3.68 (m, 2H), 3.62-3.59 (m, 6H), 3.54-3.52 (m, 2H), 3.37 (s, 3H), 2.45 (s, 3H).

**Compound 4:** A suspension of compound 2 (7.5 g, 0.024 mol), 3 (3 g, .011 mol), and potassium carbonate (6.2 g, 0.045 mol) in DMF (30 ml) was heated to 90 °C for 12 hours, under nitrogen atmosphere. The reaction mixture cooled to room temperature, diluted with dichloromethane and filtered to remove solid residue. The solution was washed from excess water, dried over MgSO<sub>4</sub> and concentrated in vacuum. The obtained crude oil further purified from silica gel column chromatography (EtOAc/PE) (4g, 64%). <sup>1</sup>H NMR (500 MHz, CDCl<sub>3</sub>) δ 7.15 (s, 2H), 4.13 (t, 4H), 3.88-3.86 (m, 4H), 3.78-3.77 (m, 4H), 3.69-3.66 (m, 8H), 3.57-3.55 (m, 4H), 3.38 (s, 6H).

**PB2T-TEG:** The monomers 4 (0.17 g, 0.30 mmol) and 5 (0.15 g, 0.30 mmol) were dissolved in 5 ml of toluene, purged with nitrogen to remove oxygen. The catalyst Pd(PPh<sub>3</sub>)<sub>4</sub> (14 mg) was added into the reaction mixture, purged again for several minutes. The reaction mixture temperature was raised to 110 °C and stirred for 12 hours under nitrogen atmosphere. The reaction mixture was cooled to room temperature, the crude polymer precipitated in hexane, further purified by soxhlet extraction with methanol, hexane and chloroform (0.13 g, 75%). <sup>1</sup>H NMR (400 MHz, CDCl<sub>3</sub>) δ 7.53 (d, J = 3.5 Hz, 2H), 7.29 (d, J = 10.0 Hz, 2H), 7.21 (s, 2H), 4.37 – 4.27 (m, 4H), 4.01 (t, J = 4.8 Hz, 4H), 3.81 (dd, J = 5.5, 3.6 Hz, 4H), 3.76 – 3.70 (m, 4H), 3.66 (dd, J = 5.5, 3.7 Hz, 4H), 3.54 (dd, J = 5.6, 3.6 Hz, 4H), 3.36 (s, 6H).

**Electrochemical, thermal, and optical properties of PB2T-TEG.** Cyclic voltammetry (CV) was done on a CHI600A electrochemical workstation with Pt disk, Pt plate, and standard calomel electrode (SCE) as working electrode, counter electrode, and reference electrode, respectively, in a 0.1 M Bu<sub>4</sub>NPF<sub>6</sub> acetonitrile

solution. The CV curves were recorded versus the potential of SCE at the scan rate of 100 mV/s, which was calibrated by the ferrocene-ferrocenium (Fc/Fc<sup>+</sup>) redox couple (5.1 eV below the vacuum level). CV was used to measure the energy levels, as depicted in **Figure S1**. The HOMO energy level was calculated from onset oxidation potential, according to the equation  $E_{\text{HOMO}} = -[(E_{\text{ox}}^{\text{onset}} - E_{1/2}(\text{Ferrocene}))]$ . Whereas, the LUMO energy levels were estimated by using the equation  $E_{\text{LUMO}} = [E_{\text{g}}^{\text{opt}} + E_{\text{HOMO}}]$ . The data are summarized in **Table S1**. UV-vis absorption spectra were recorded on a Shimadzu UV-2450 spectrophotometer. The UV-vis absorption properties of the polymer determined in chlorobenzene and thin film (spin cast onto glass substrate) as shown in **Figure S1** and characteristic data are summarized in **Table S1**. Both absorption spectra showed two characteristics peaks in the main absorption band range (400-600 nm). A small red shift with increase in the vibronic peak intensity observed in the thin film absorption spectra, suggested an increase in aggregation from solution to film. Thermogravimetric analysis (TGA) was carried out on a WCT-2 thermal balance under nitrogen atmosphere at a heating rate of 10 °C/min, and it was heated from room temperature to 600 °C. The thermal decomposition ( $T_d$ ) at 5% weight loss was observed at 267 °C as shown in **Figure S2**. The molecular weight and molecular weight distribution were determined with a PL-GPC220 chromatograph, which was calibrated to polystyrene standards. The GPC columns were eluted with THF with 1.0 ml/min at 40 °C, and the sample concentration was 2 mg/ml.

### Synthesis of P3MEEMT

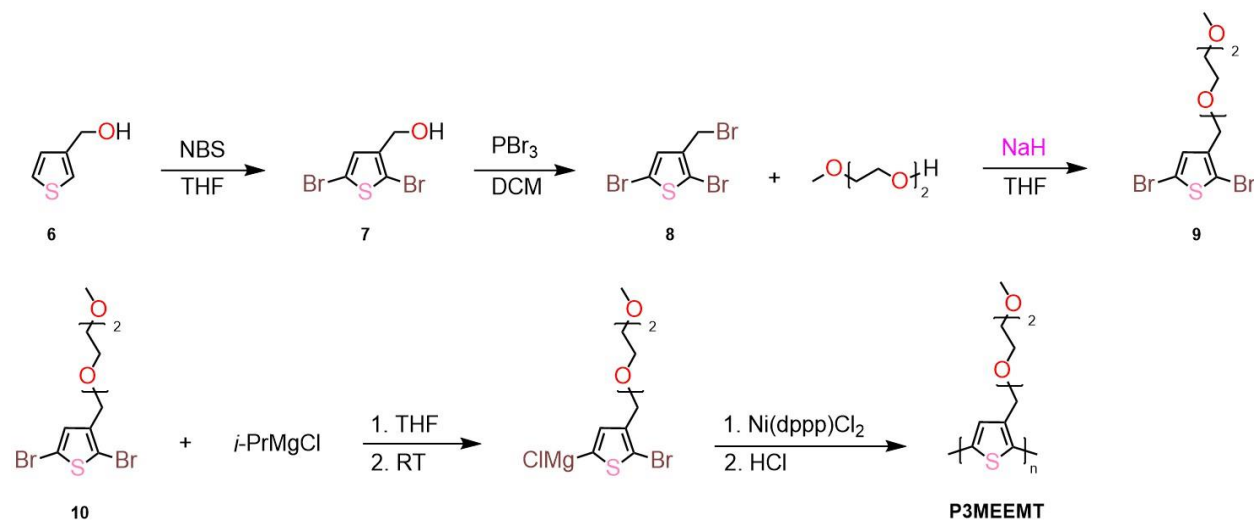

**Scheme 2.** Synthetic procedure for monomer 9 and polymer P3MEEMT.

P3MEEMT was synthesized as previously described.<sup>1,2</sup> The procedure will be described in detail herein.

**Compound 7:** To a dried 3-neck flask, 6 (3.77 mL, 40 mmol) and 36.4 mL of THF was added, and the solution was degassed under nitrogen bubbling for 15 minutes. After degassing, 5 equal portions of recrystallized NBS (total: 14.15g, 79.5 mmol) were added to the reaction, capping the flask in between additions. The reaction was covered with foil, and allowed to stir overnight under N<sub>2</sub>. The reaction was then rotovapped, suspended with hexanes, and filtered through a frit to remove solids. The hexanes was then removed through rotovapping, and the residue purified through column chromatography using a 4:1 ratio of hexanes:ethyl acetate. Product was recovered as a white solid in 90% yield. <sup>1</sup>H NMR (300 MHz, CDCl<sub>3</sub>):  $\delta$  7.03 (s, 1H), 4.60 (s, 2H), and 1.95 (br, 1H).

**Compound 8:** To a dried round bottom flask, 7 (9.0 g, 33.5 mmol) and 165 mL of anhydrous DCM was added, then cooled to 0 °C for 20 min. PBr<sub>3</sub> (3.20 mL, 34.25 mmol) was added dropwise over 15 min, maintaining a 0 °C temperature. The reaction was then allowed to warm to room temperature, and stirred for 5 h, after which it was quenched by the addition of 100 mL of 10% NaHCO<sub>3</sub> solution. Once bubbling

had subsided, the product was extracted with DCM. The organic layer was collected, and washed with brine, then dried over  $\text{MgSO}_4$  and filtered. The DCM was removed using rotary evaporation, after which the product was stored at  $-20\text{ }^\circ\text{C}$  overnight, resulting in the formation of a white solid in 93% yield.  $^1\text{H}$  NMR (300 MHz,  $\text{CDCl}_3$ ):  $\delta$  7.00 (s, 1H), 4.36 (s, 2H).

**Compound 9:** To a dried 3-neck flask equipped with an addition funnel, diethylene glycol monomethyl ether (3.5 mL, 30 mmol) and 100 mL of anhydrous THF was added under  $\text{N}_2$ . A 60% suspension of NaH in mineral oil (1.32 g, 33 mmol) was quickly added in one portion, and the flask was sealed to  $\text{N}_2$ , taking care not to allow the flask to pressurize with  $\text{H}_2$ . The NaH was allowed to react for 10 minutes, then 8 (9.65 g, 29 mmol) and 25 mL of THF were added to the addition funnel. 8 was added dropwise from the funnel over 15 minutes, then the reaction was allowed to stir at room temperature overnight. The reaction mixture was filtered over a thin pad of Celite, and the product washed through with THF. Solvent was removed using rotary evaporation. The residue was purified using column chromatography, with a 3:2 mixture of hexanes:ethyl acetate as the eluent. The product was collected in 87% yield as a pale yellow oil. The product was stored at  $-20\text{ }^\circ\text{C}$  covered from light.

**P3MEEMT Synthesis:** 9 (0.370 g, 1.0 mmol) was added to a dried Schlenk flask under  $\text{N}_2$ , then degassed under high vacuum for 30 min. After degassing, the flask was returned to an  $\text{N}_2$  environment, and 10 mL of anhydrous THF was added. The flask was cooled on ice to  $0\text{ }^\circ\text{C}$ , after which *i*-PrMgCl (2.0 M in THF, 0.5 mL, 1.0 mmol) was added dropwise over 10 min, then the flask was allowed to warm to room temperature and stirred for 1 h. The flask was heated to  $45\text{ }^\circ\text{C}$  and the  $\text{Ni(dppp)Cl}_2$  (4.334 mg, 0.008 mmol) was added quickly and in one portion. The polymerization was allowed to continue for 2 h at  $45\text{ }^\circ\text{C}$ , after which it was quenched by the addition of HCl (5 M, 1 mL). The polymer was then precipitated into 400 mL of MeOH, and collected over a filter. The polymer was purified using successive Soxhlet extractions in hexanes and MeOH, then collected with  $\text{CHCl}_3$ . The polymer was precipitated again into MeOH and collected over a filter, then dried overnight in a vacuum oven.  $^1\text{H}$  NMR (500 MHz,  $\text{CDCl}_3$ )  $\delta$  7.25 (s, 1H), 4.67 (s, 2H), 3.75 (s, 4H), 3.67 (m, 2H), 3.57 (m, 2H), 3.37 (s, 3H).  $\bar{D} = 2.0$ ,  $M_n = 11\text{ kg/mol}$ . The SEC experiment was done using THF as an eluent, at 1 mL/min flow rate with a Viscotek TDA305 detector array. The samples were run at  $40\text{ }^\circ\text{C}$ , and molecular weights were determined by comparison against polystyrene standards.

**Electrochemical measurements in aqueous electrolytes.** Electrochemical measurements were performed with a Metrohm Autolab PGSTAT204 with NOVA Software (2.1.4). A Pt wire was used as the counter electrode (Aldrich) and an Ag/AgCl electrode (Harvard Apparatus Ltd.) was used as the reference electrode for all measurements. Cyclic voltammetry was acquired in the range of  $-0.5$  to  $+0.7\text{ V}$  (vs. Ag/AgCl) at a rate of  $0.1\text{ V/s}$  in 100 mM KCl or 100 mM  $\text{KPF}_6$  (degasses for 20 min by bubbling  $\text{N}_2$  before using).

**Spectroelectrochemistry of doping kinetics.** Spectroelectrochemistry measurements were acquired using an Agilent 8453 spectrometer. PB2T-TEG ( $\sim 100\text{ nm}$ ) was spin coated onto glass coated with fluorine-doped tin oxide (FTO) substrates (Aldrich). A series of spectra were acquired through the NOVA Software during doping and dedoping in degassed 100 mM KCl at a range of 0 to  $+0.7\text{ V}$  vs. Ag/AgCl for 120 s once the bias was applied with 100 ms/spectrum integration time. The decrease in absorption was fit to a biexponential decay in Matlab.

**Electrochemical quartz crystal microbalance (EQCM).** Electrogravimetric measurements were performed using a QCM200 (Stanford Research Systems) on 5 MHz gold-coated AT quartz crystals. Measurements were collected with a three-electrode cell with the PB2T-TEG-coated crystal face functioning as the working electrode. The change in frequency was converted to a change in mass using the Sauerbrey equation.

**X-ray diffraction (XRD).** Samples for XRD were spin coated on FTO-coated glass (Aldrich) and annealed for 20 min at 160 °C in N<sub>2</sub>. Samples of P3HT (Ossila, M106), P3MEEMT, and PB2T-TEG were doped at a range of voltages (0-0.7 V vs. Ag/AgCl) in 100 mM KCl (or 100 mM KPF<sub>6</sub> for P3HT). XRD diffraction patterns were obtained using a Bruker D8 Discover with a Pilatus 100K large-area 2D detector. 2D data was acquired from 2 to 13 2 $\theta$  and an integration time of 120 s per step. Line cuts were plotted using polar integration of the 2D maps. The (100) peaks were fit with a single Gaussian to determine the peak position.

**Grazing incidence wide angle scattering (GIWAXS).** GIWAXS measurements were performed on Beamline 7.3.3 at the Advanced Light Source (ALS) at Lawrence Berkeley National Lab using a Pilatus 2M area detector and an incidence angle of 0.18° with 30 s exposure times. Data was processed using Nika and WAXStools<sup>3</sup> in Igor Pro 7. *In operando* GIWAXS measurements were acquired using a custom-made liquid cell (see **Figure S8** for images of the liquid cell) on the same beamline with an incidence angle of 2°. The cell is composed of a 12.7  $\mu$ m-thick polyimide window (TF-412, Premier Lab Supply) coated with 5 nm Cr and 30 nm Au using an Edwards Auto 306 thermal evaporator. The Au-coated polyimide film is coated with ~100 nm of polymer with spin coating. The liquid cell uses a PDMS spacer (Dow SYLGARD 184 Kit) and an Ag/AgCl counter electrode (eDAQ) between the polyimide/Au/polymer film and a glass slide. Aqueous electrolyte is injected between the glass and polymer film using a needle prior to measurement. The voltage was applied using a Keithley source measure unit (Keithley 2400 SourceMeter, Tektronix).

**Optical transmission imaging.** Optical transmission images of doped/undoped interfaces were acquired using an EVOS M7000 microscope (Thermo Fischer) using a 750  $\pm$  25 nm bandpass filter to capture the polaron absorption. To fabricate the half-doped samples, the polymer (PB2T-TEG or P3MEEMT) was spin-coated onto an ITO-coated glass substrate. Half of the substrate was electrochemically doped by submerging half of the substrate in 100 mM KCl or KPF<sub>6</sub> and applying a +0.7 V (vs. Ag/AgCl) bias to drive ions into the polymer film. Transmission images were captured with several minutes to hours between acquisitions to capture the progression of the interface.

**Photoinduced force microscopy (PiFM).** Polymer samples for PiFM were fabricated following the same procedure as the optical transmission imaging. A Molecular Vista VistaScope coupled to a LaserTune QCL was used for imaging. The laser was tuned to the P-F vibration of PF<sub>6</sub><sup>-</sup> at 843 cm<sup>-1</sup> for image acquisition. A time series of 256 x 256 pixel images were acquired with a 20 x 20 or 3 x 3  $\mu$ m field-of-view with a scan rate of 1 s/line. The same field-of-view was scanned many times to build up movies of ion front motion. Both topography and PiFM images were processed in Matlab.

## Supplementary Text on Diffusion Calculations

Ion diffusion in PB2T-TEG and P3MEEMT were modeled using numerical calculations of the one-dimensional diffusion equation.

$$\frac{\delta x}{\delta t} = \frac{\delta}{\delta y} \left( D \frac{\delta x}{\delta y} \right)$$

Where  $x$  is local concentration of ions,  $t$  is the time,  $D$  is the diffusion constant, and  $y$  is the spatial coordinate. This equation can be expressed in terms of finite derivatives:<sup>4</sup>

$$\begin{aligned} \frac{x(y, t + \delta t) - x(y, t)}{\delta t} = & \left( \frac{D(x, y + \delta y, t) - D(x, y - \delta y, t)}{2\delta y} \right) \left( \frac{x(y - \delta y, t) - x(y + \delta y, t)}{2\delta y} \right) \\ & + D(x, y, t) \left( \frac{x(y + \delta y, t) - 2x(y, t) + x(y - \delta y, t)}{(\delta y)^2} \right) \end{aligned}$$

We define the diffusion constant as a combination of the diffusion constant in the oxidized, expanded lattice ( $D_{ox}$ ) and the diffusion constant of the neutral polymer with a contracted lattice ( $D_{neut}$ ). The concentration-dependent form of  $D$  is not known, so we choose a function form that approximates the data. Here, we use:

$$D(x) = (D_{ox} - D_{neut})x^4 + D_{neut}$$

This equation satisfies the boundary conditions that if  $x = 0$ , the diffusion constant is  $D_{neut}$  and if  $x = 1$ , the diffusion constant is  $D_{ox}$ . For  $D_{ox} = D_{neut}$ , typical concentration-independent Fickian diffusion occurs. We plot the resulting concentration profiles as a function of time in **Figure S14** for  $D_{ox} = D_{neut}$ ,  $10 \times D_{neut}$ ,  $100 \times D_{neut}$ , and  $1000 \times D_{neut}$ , as well as the data converted into % transmission to more easily compare to the experimental data in **Figure S12**. As the relative difference between  $D_{ox}$  and  $D_{neut}$  increases, the interface profile becomes sharper. Qualitatively, the concentration profiles at  $D_{ox} = D_{neut}$  or  $10 \times D_{neut}$  more closely match the experimentally-determined profiles of P3MEEMT, suggesting that ion motion is limited by the intrinsic diffusivity of the ions. The concentration profiles at  $D_{ox} = D_{neut}$  most closely match the experimentally-determined profiles of PB2T-TEG, maintaining a sharp phase front upon interface migration. Additionally, the calculations, as well as the experiment, show a deceleration of the phase front over time. Overall, the calculations show that the sharp phase front could be an extreme example of concentration-dependent diffusion.

## Supplementary Figures

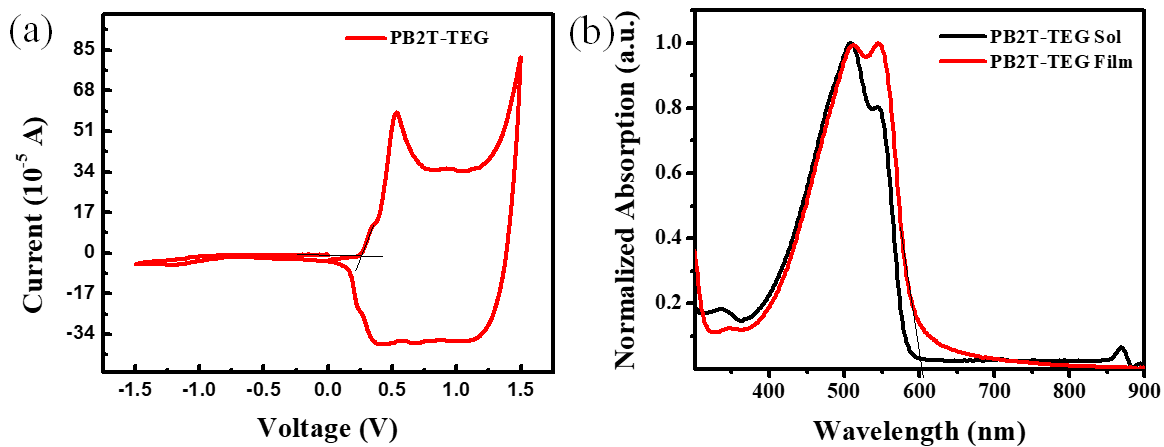

**Figure S1:** (a) Cyclic voltammogram and of PB2T-TEG in a 0.1 M  $\text{Bu}_4\text{NPF}_6$  acetonitrile solution scanning at 100 mV/s (b) normalized UV-vis absorption spectra of PB2T-TEG in chlorobenzene and as a thin film on glass.

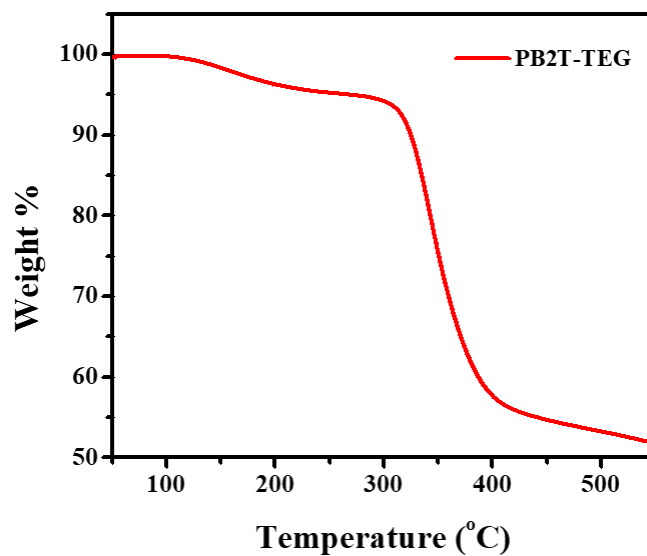

**Figure S2:** Thermogravimetric analysis plot of PB2T-TEG.

**Table S1.** Optical properties, energy levels, and molecular weight of PB2T-TEG

| Polymer  | $\lambda_{\max}^a$<br>(nm) | $\lambda_{\max}^b$<br>(nm) | $\lambda_{\text{onset}}^b$<br>(nm) | $\epsilon$ ( $10^4$<br>$M^{-1}$<br>$cm^{-1}$ ) <sup>a</sup> | $E_g^{\text{opt}}$<br>(eV) | $E_{\text{onset}}^{\text{ox}}$<br>(V) | $E_{\text{HOMO}}$<br>(eV) | $E_{\text{LUMO}}$<br>(eV) | $M_n^c$<br>kg/mol | $M_w$<br>Kg/mol | $D$ |
|----------|----------------------------|----------------------------|------------------------------------|-------------------------------------------------------------|----------------------------|---------------------------------------|---------------------------|---------------------------|-------------------|-----------------|-----|
| PB2T-TEG | 510                        | 547                        | 603                                | 3.45                                                        | 2.05                       | 0.25                                  | -4.63                     | -2.32                     | 8.9               | 9.7             | 1.1 |

<sup>a</sup> The data was measured from chlorobenzene solution, <sup>b</sup> the data was measured from a thin film, <sup>c</sup> GPC was measured from tetrahydrofuran solution.

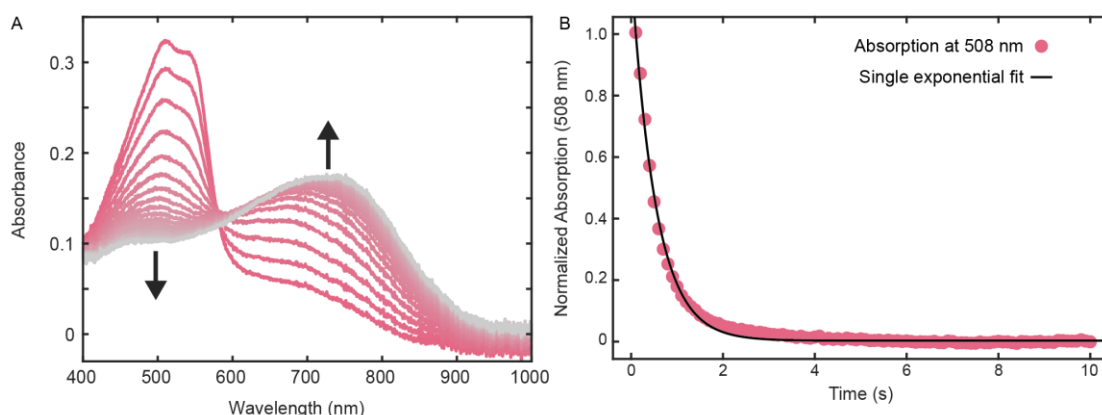

**Figure S3: UV-Vis spectra of PB2T-TEG as a function of time upon applying a +0.7 V bias.** (A) A series of absorption spectra with time upon applying a +0.7 V bias with 0.1 s integration time between each spectrum on a 100 nm thick PB2T-TEG thin film on FTO. (B)  $\pi$ - $\pi^*$  absorption peak max (508 nm) as a function of time fit with a single exponential decay. The time constant from the single exponential decay is  $530 \pm 20$  ms.

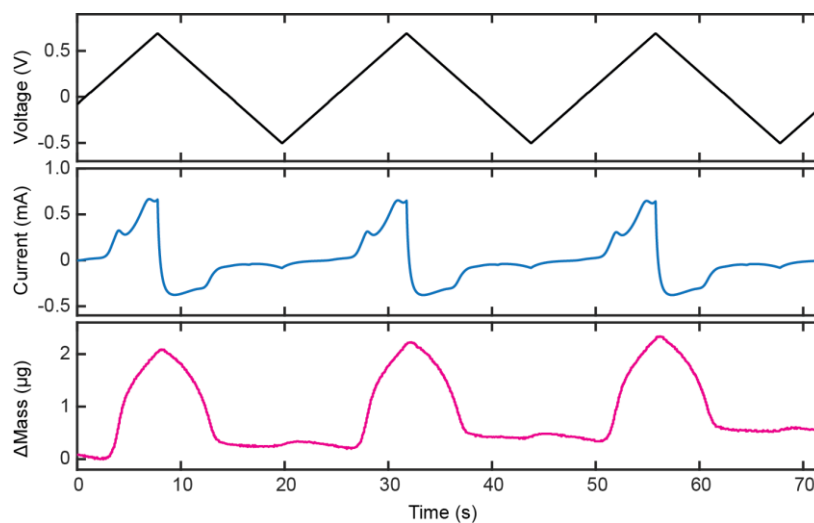

**Figure S4: Electrochemical quartz crystal microbalance (EQCM) of PB2T-TEG (100 nm thickness) in 100 mM KCl.** The applied voltage (vs. Ag/AgCl), measured current, and change in mass are shown.

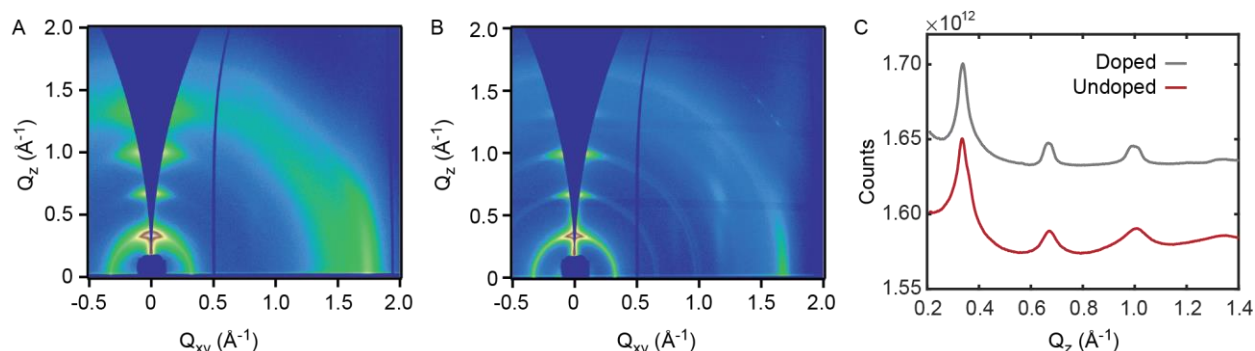

**Figure S5: Undoped and doped GIWAXS diffraction patterns of P3MEEMT.** (A) GIWAXS diffraction pattern of undoped P3MEEMT. (B) GIWAXS diffraction pattern of doped P3MEEMT (0.7 V vs. Ag/AgCl in 100 mM KCl). (C) Out-of-plane line-cuts showing no significant change in the lamellar spacing upon electrochemical doping.

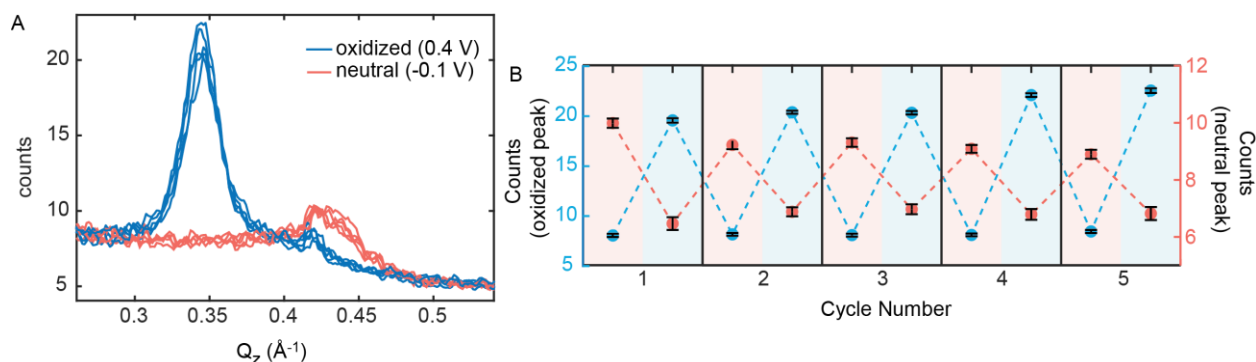

**Figure S6: XRD patterns of PB2T-TEG alternating between -0.1 V and +0.4 V (vs. Ag/AgCl) to show reversibility of the structural phase transition.** (A) XRD patterns alternating between oxidized (blue) and neutral (red) of PB2T-TEG. (B) Oxidized and neutral peak intensities over five cycles of oxidation and reduction.

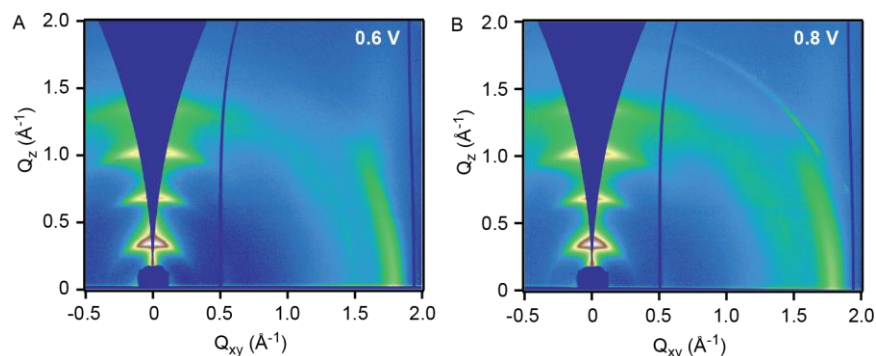

**Figure S7: GIWAXS diffraction patterns of PB2T-TEG at higher doping potentials.** GIWAXS patterns at (A) +0.6 V and (B) +0.8 V (vs. Ag/AgCl).

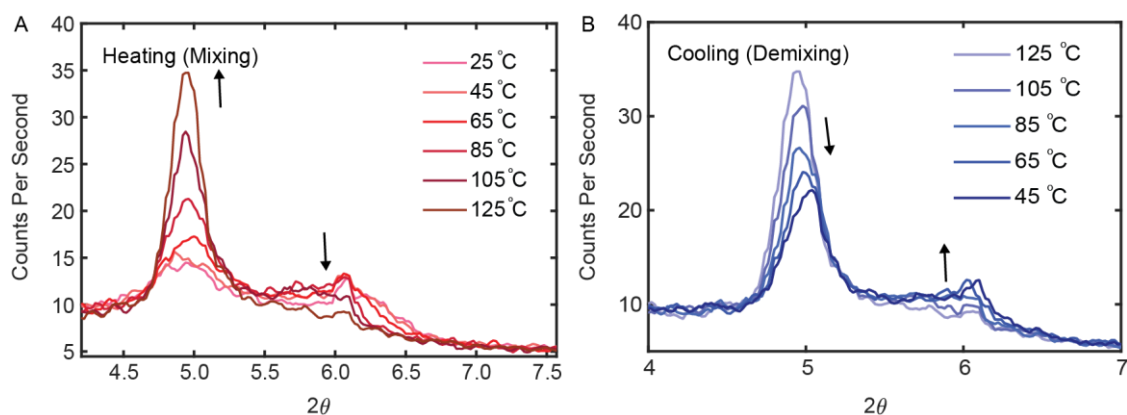

**Figure S8: Temperature-dependent XRD of PB2T-TEG.** (A) Heating a phase-separated PB2T-TEG film (doped at +0.23 V) with XRD patterns recorded at a number of temperatures. The undoped peak becomes less intense with temperature, signifying mixing of the ions. (B) Cooling of the same PB2T-TEG sample, showing a demixing of the ions as the doped peak decreases in intensity and the undoped peak increases in intensity.

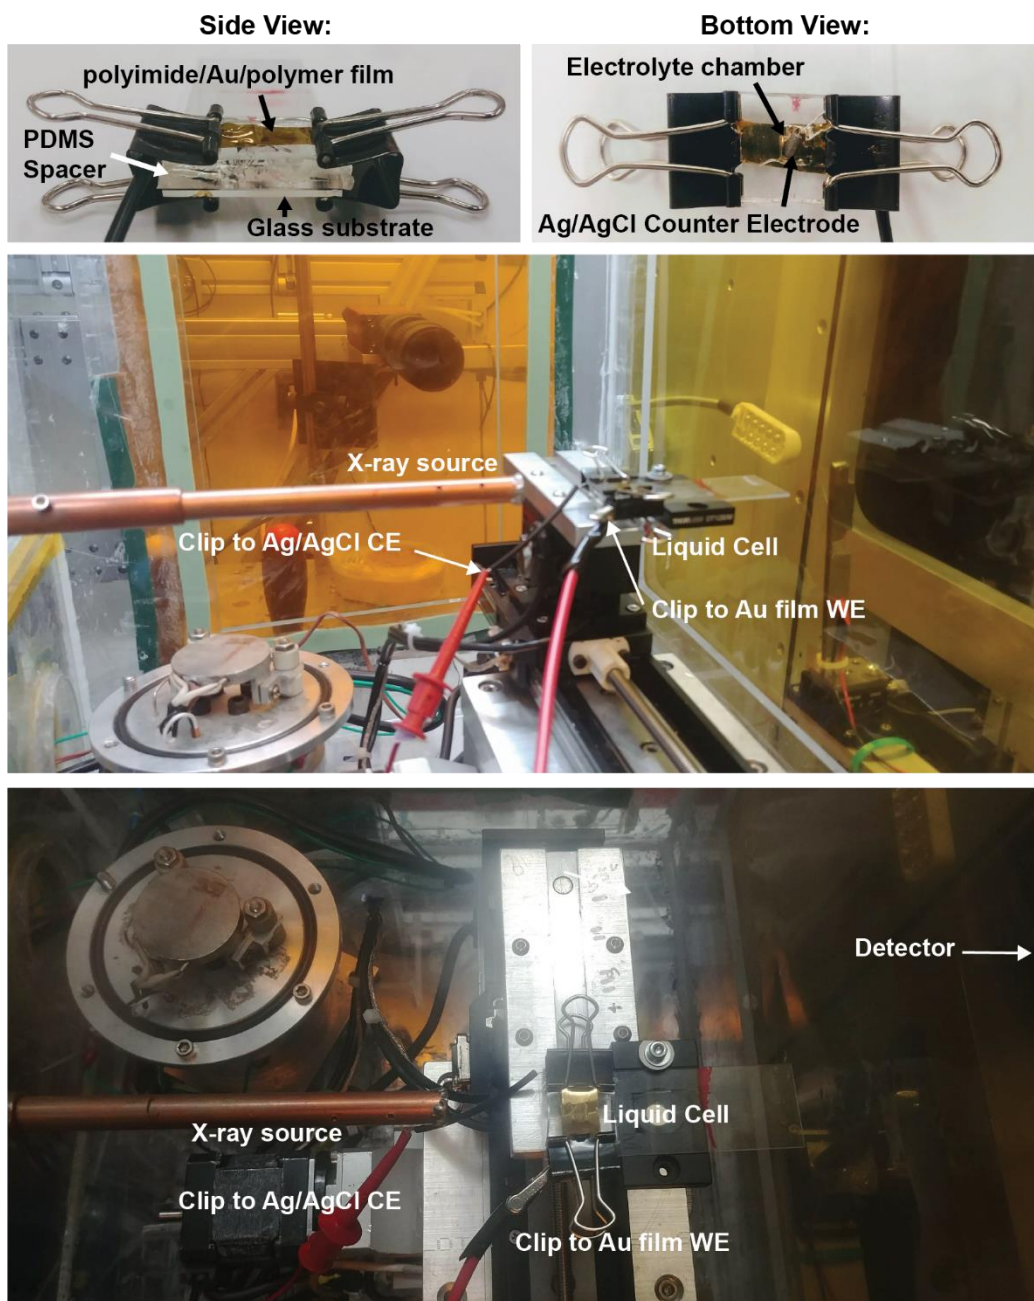

**Figure S9:** Additional images of the *in operando* liquid cell.

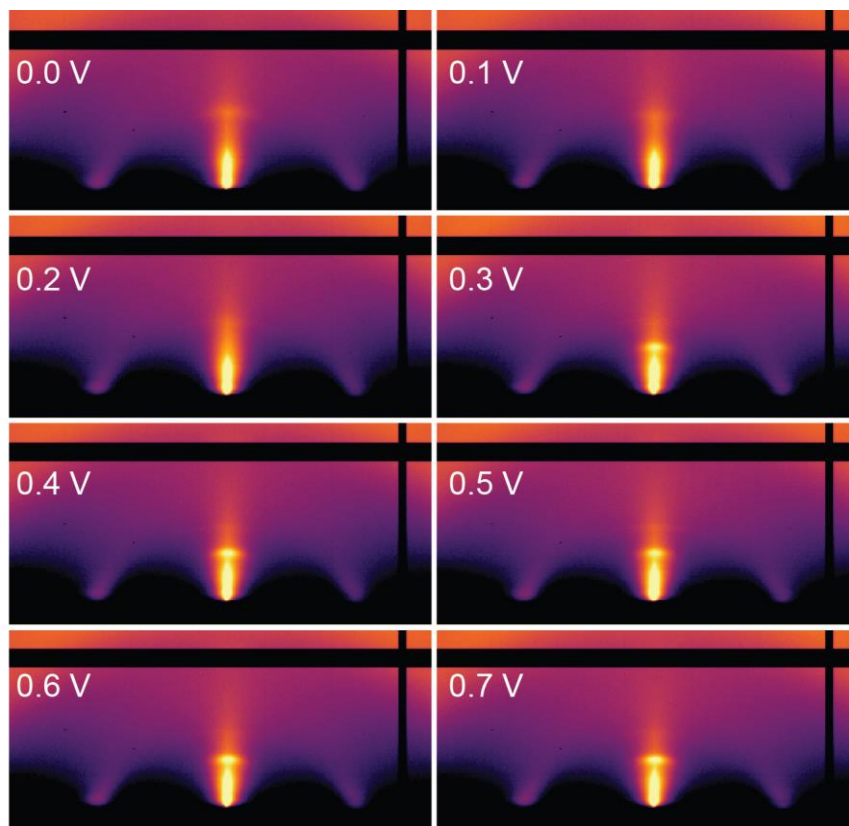

**Figure S10:** *In operando* GIWAXS patterns of PB2T-TEG as a function of applied bias. GIWAXS diffraction patterns are collected at voltages ranging from 0.0 to +0.7 V.

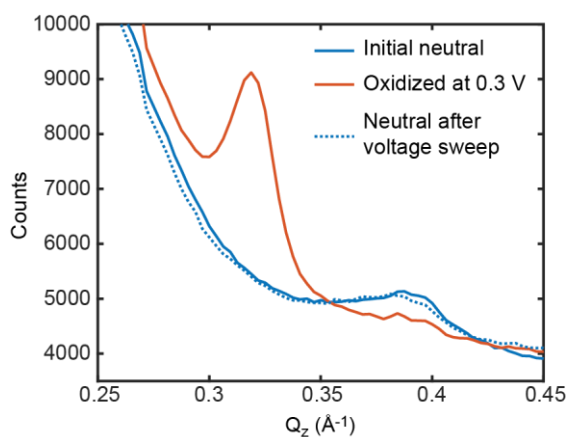

**Figure S11: Reversibility *in operando*.** Diffraction pattern linecuts showing the reversibility of the phase transition when using the liquid cell. The diffraction peak corresponding to the neutral polymer reappears after a voltage sweep from 0 to +0.7 V (vs. Ag/AgCl) and the peak corresponding to the oxidized polymer disappears.

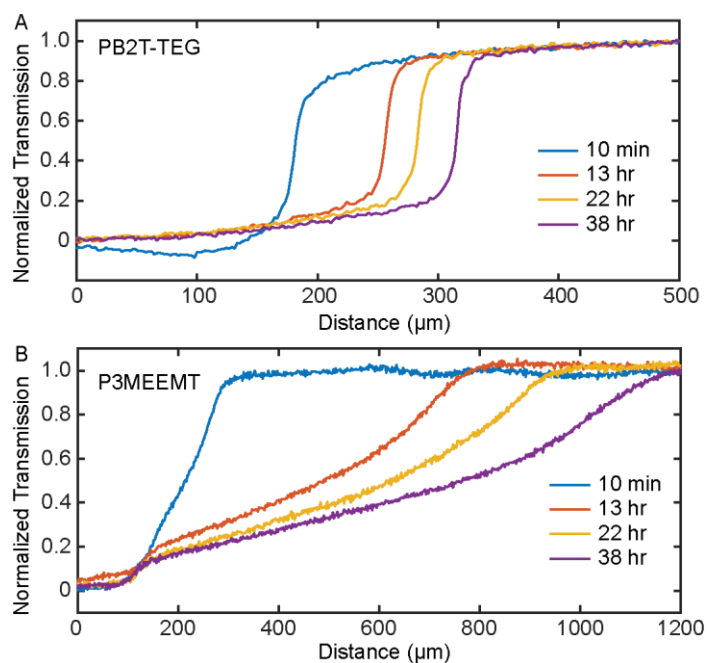

**Figure S12: Line cuts of optical transmission images of ion front motion.** Line cuts of (A) PB2T-TEG and (B) P3MEEMT at 10 min, 13 hr, 22 hr, and 38 hr. The interface between doped and undoped regions of P3MEEMT spreads out with time, where the interface between doped and undoped regions of PB2T-TEG remains sharp.

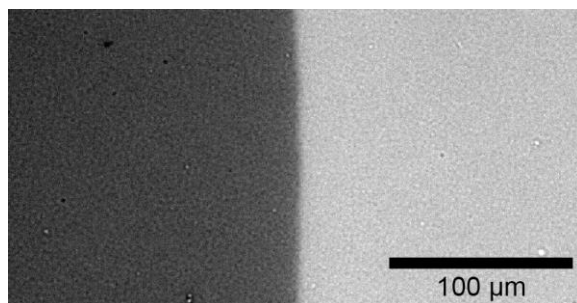

**Figure S13: Image of PB2T-TEG ion front 6 months after doping.** The image was acquired with a  $750 \pm 20$  nm bandpass filter. The dark region is oxidized.

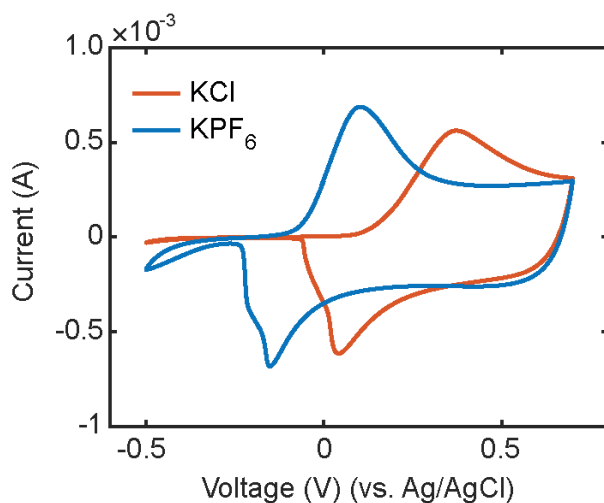

**Figure S14:** Cyclic voltammetry (CV) of PB2T-TEG with 100 mM KCl and 100 mM KPF<sub>6</sub> showing the shift in threshold voltage when using PF<sub>6</sub><sup>-</sup>.

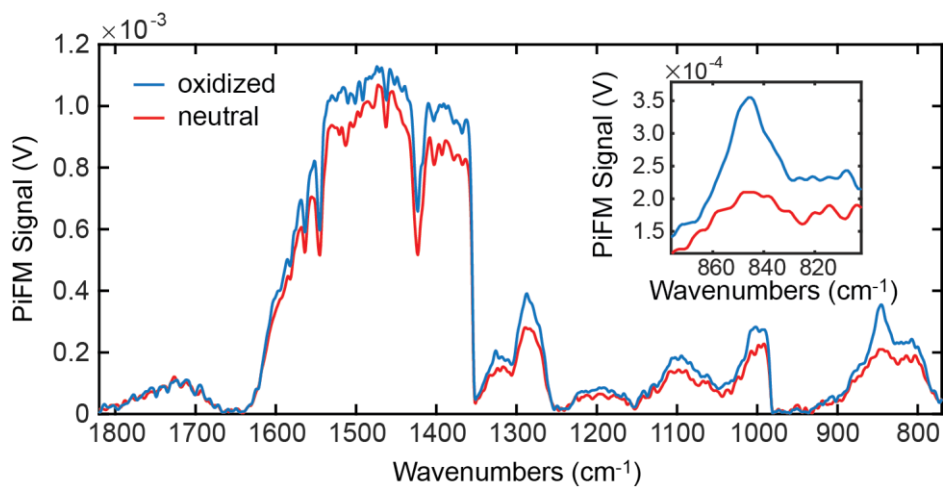

**Figure S15:** PiFM spectra of neutral and electrochemically oxidized PB2T-TEG with KPF<sub>6</sub> (0.7 V vs. Ag/AgCl). The peak corresponding to the P-F vibration of PF<sub>6</sub><sup>-</sup> is at ~843 cm<sup>-1</sup>. The inset shows the peak corresponding to PF<sub>6</sub><sup>-</sup>.

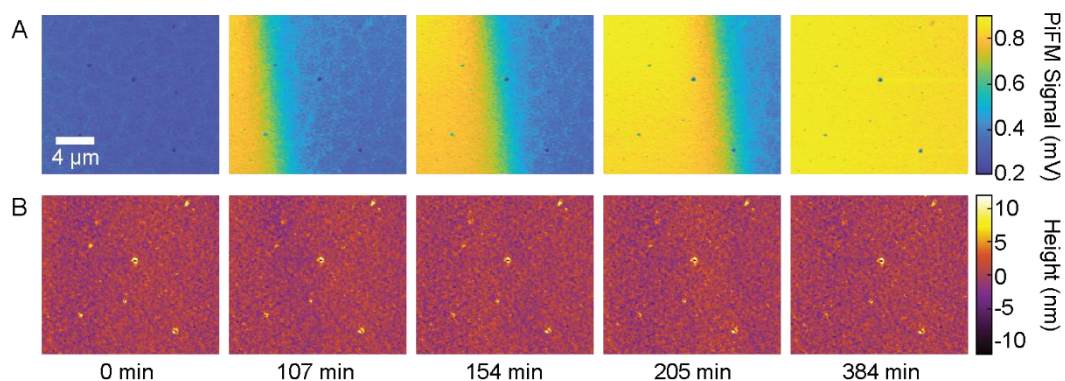

**Figure S16: PiFM of larger field-of-view and line-cut showing a sharp interface in PB2T-TEG.** (A) Time series of PiFM images with a 20 x 20  $\mu\text{m}$  field-of-view of an ion front migrating. (B) Time series of topography images spatially correlated to the PiFM images. Changes in the topography are difficult to see at this length scale.

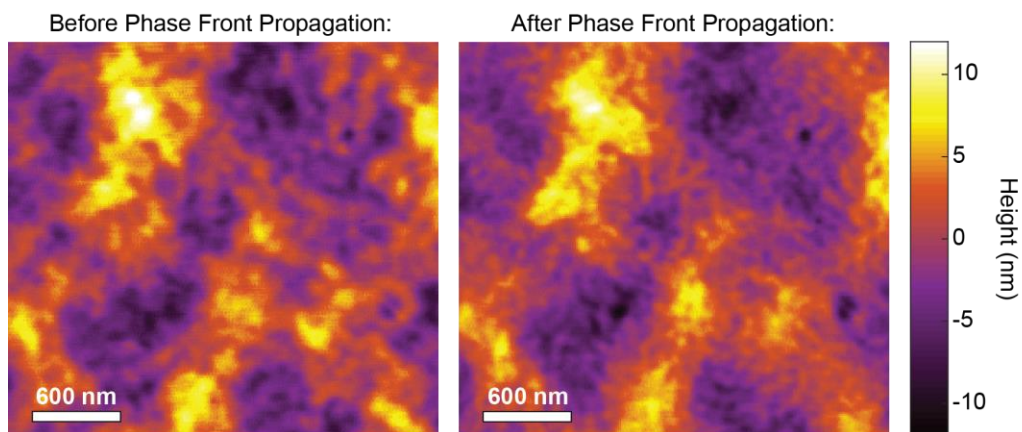

**Figure S17: Topography of PB2T-TEG before and after ion front propagation.**

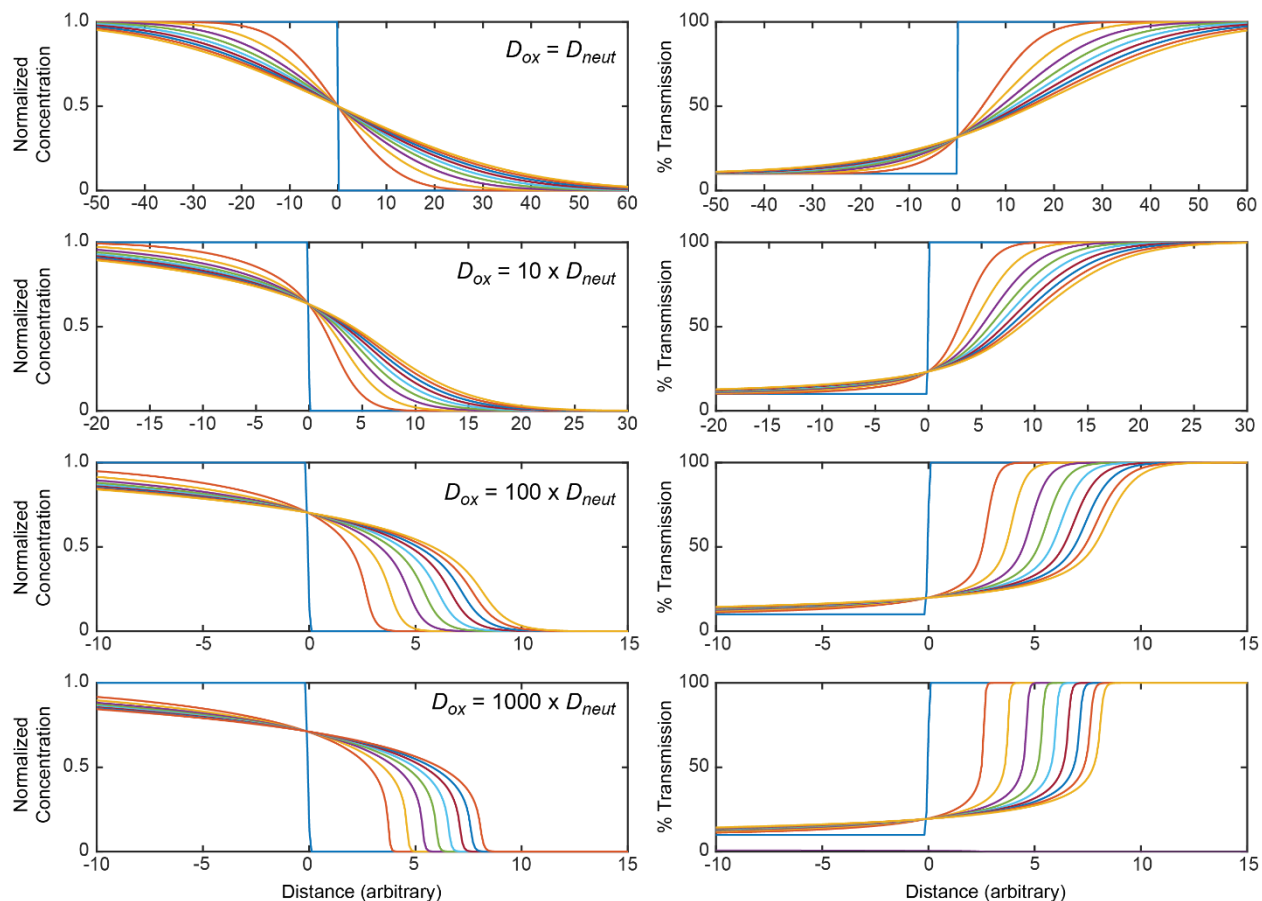

**Figure S18: Results of concentration-dependent diffusion calculations.** Results of diffusion calculations show how the interface migration depends on the difference in diffusion constants in the oxidized and neutral regions of the polymer. The blue step function shows the initial concentration profile.

### Supplementary Movie Captions

**Movie S1: Optical moving front experiment.** A time series of transmission images of the moving front experiment for PB2T-TEG and P3MEEMT with associated line-cuts. The sharp line that remains constant in time in the P3MEEMT film is presumably from an immobile fraction of ions.

**Movie S2: PiFM of the moving front in a 3 x 3  $\mu\text{m}$  field-of-view.** Correlated topography and PiFM images of the ion front using the P-F vibration of  $\text{PF}_6^-$  as the contrast.

**Movie S3: PiFM of the moving front in a 20 x 20  $\mu\text{m}$  field-of-view.** Correlated topography and PiFM images of the ion front using the P-F vibration of  $\text{PF}_6^-$  as the contrast.

### Supplementary References:

1. Flagg, L. Q., Bischak, C. G. & Ginger, D. S. Polymer Crystallinity Controls Water Uptake in Glycol Side Chain Polymer Organic Electro-chemical Transistors. *J. Am. Chem. Soc.*
2. Dong, B. X. *et al.* Influence of Side-Chain Chemistry on Structure and Ionic Conduction Characteristics of Polythiophene Derivatives: A Computational and Experimental Study. *Chem. Mater.* **31**, 1418–1429 (2019).
3. Oosterhout, S. D. *et al.* Mixing Behavior in Small Molecule:Fullerene Organic Photovoltaics. *Chem. Mater.* **29**, 3062–3069 (2017).
4. Harrison, P. Numerical solution to the general one-dimensional diffusion equation in semiconductor heterostructures. *Phys. Status Solidi B* **197**, 81–90 (1996).
